# Supplementary material for: Resonant band hybridization in alloyed transition metal dichalcogenide heterobilayers
Source: arXiv:2309.13312 ancillary file (2023-09-23)
Supplement: Supplementary file 1 [file Supp_Info.pdf]

# Supporting information for Resonant band hybridization in alloyed transition metal dichalcogenide heterobilayers

A. Catanzaro[1], A. Genco[1,2*], C. Louca[1,2], D. A. Ruiz-Tijerina[3], D. J. Gillard[1], L. Sortino[1,4], A. Kozikov[5,6], E. Alexeev[1,7], R. Pisoni[8], L. Hague[9], K. Watanabe[10], T. Taniguchi[11], K. Ensslin[8], K. S. Novoselov[12], V. Fal'ko[5], and A. I. Tartakovskii[1**]

[1]*Department of Physics and Astronomy, University of Sheffield, Sheffield S3 7RH, UK*

[2]*Dipartimento di Fisica, Politecnico di Milano, Piazza Leonardo da Vinci, 32, Milano, 20133, Italy*

[3]*Departamento de Física Química, Universidad Nacional Autónoma de México, Ciudad de México, C.P. 04510, México*

[4]*Chair in Hybrid Nanosystems, Nanoinstitute Munich, Faculty of Physics, Ludwig-Maximilians-Universität München, Munich, Germany*

[5]*Department of Physics and Astronomy, University of Manchester, Manchester M13 9PL, UK*

[6] *School of Mathematics, Statistics and Physics, Newcastle University, Newcastle upon Tyne, NE1 7RU, UK*

[7]*Cambridge Graphene Centre, University of Cambridge, 9 J. J. Thomson Avenue, Cambridge, CB3 0FA, UK*

[8]*Solid State Physics Laboratory, ETH Zurich, Zurich, Switzerland*

[9]*National Graphene Institute, University of Manchester, Manchester M13 9PL, UK*

[10]*Research Center for Electronic and Optical Materials, National Institute for Materials Science, 1-1 Namiki, Tsukuba 305-0044, Japan*

[11]*Research Center for Materials Nanoarchitectonics, National Institute for Materials Science, 1-1 Namiki, Tsukuba 305-0044, Japan and*

[12]*Institute for Functional Intelligent Materials, National University of Singapore, Singapore, 117546, Singapore*

∗ armando.genco@polimi.it and ∗∗ a.tartakovskii@sheffield.ac.uk

## SUPPLEMENTARY NOTE S1:. $Mo_xW_{(1-x)}Se_2$ MONOLAYERS REFLECTANCE CONTRAST

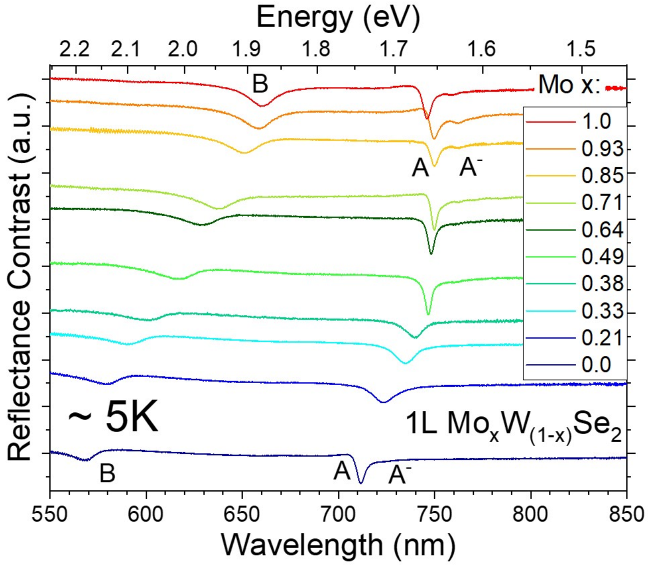


**Supplementary Figure S1**. **A and B excitons in $Mo_xW_{(1-x)}Se_2$ monolayers.** Reflectance contrast (RC) spectra measured at low temperature of isolated $Mo_xW_{(1\text{-}x)}Se_2$ alloys monolayers with different Mo concentrations ($x$). The trends of A and B excitons as a function of $x$ are clearly displayed. In some samples a small feature ascribed to the trion A- is also visible.

| Model | $(1-x)E_{Mo} + (x)E_W - bx(1-x)$ | | |
|---|---|---|---|
| **Fit Parameters** | **A** | **A$^-$** | **B** |
| **b** | 0.16 ± 0.02 | 0.15 ± 0.02 | 0.04 ± 0.05 |
| **E**$_{Mo}$ | 1.747 ± 0.004 | 1.721 ± 0.005 | 2.20 ± 0.01 |
| **E**$_W$ | 1.659 ± 0.003 | 1.632 ± 0.004 | 1.87 ± 0.01 |

TABLE S1. Model and parameters extracted from the fit of the exciton energies.

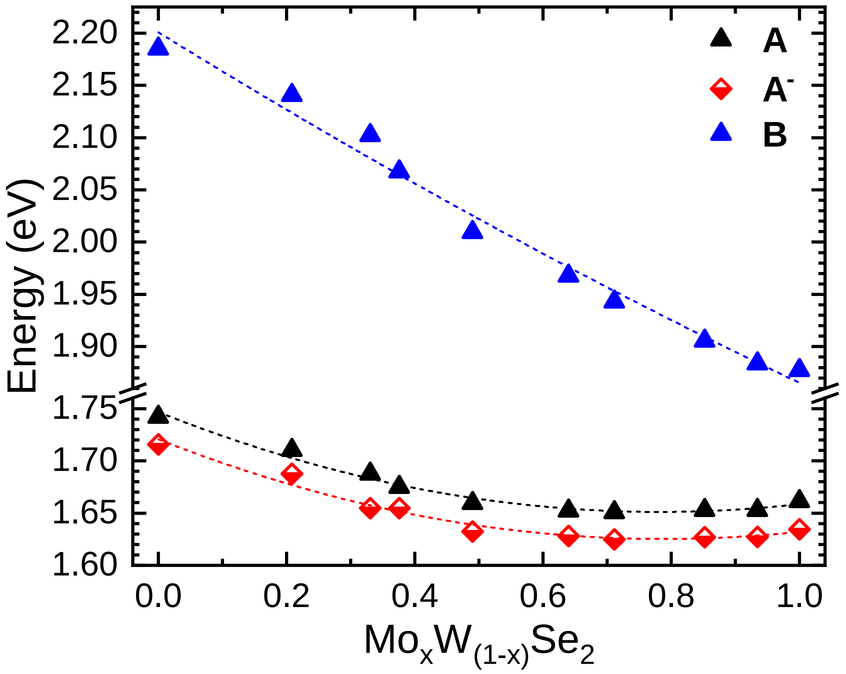


**Supplementary Figure S2. Energies of neutral A-series (A), trion (A$^-$) and B-series (B) exciton resonances on RC spectra as a function of Molybdenum concentration, $x$.** The extracted exciton energies (data-points) for each monolayer are fitted to the model shown on the table S1 with the extracted fit parameters. The fit results are shown as dashed curves

## SUPPLEMENTARY NOTE S2:. $Mo_xW_{(1-x)}Se_2$ ALLOY BILAYERS

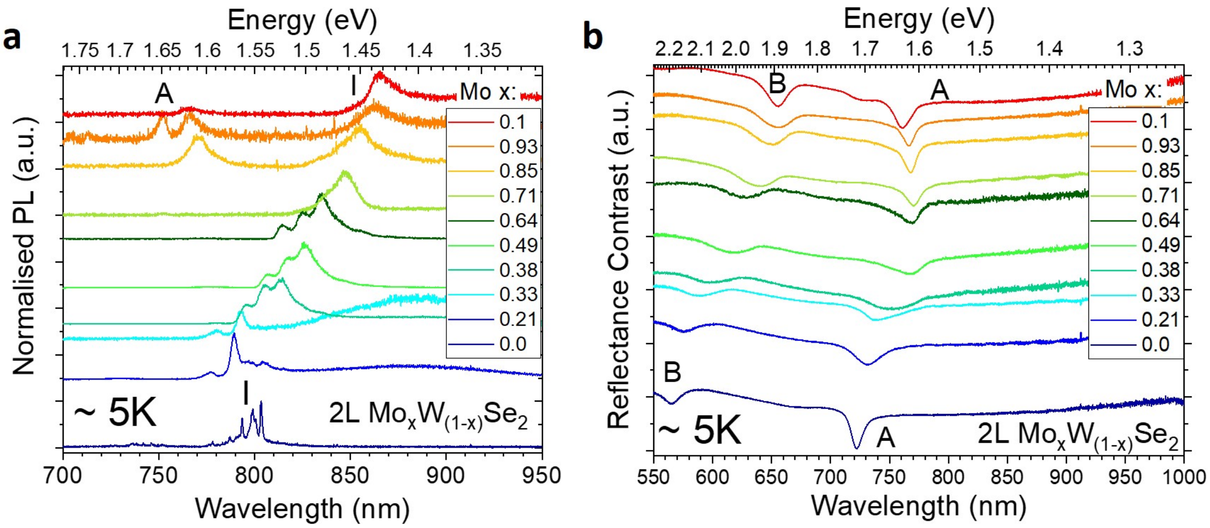


**Supplementary Figure S3**. **Excitons transitions in $Mo_xW_{(1-x)}Se_2$ alloy bilayers.a,** PL spectra measured at low temperature of isolated $Mo_xW_{(1\text{-}x)}Se_2$ alloys bilayers with different Mo concentrations ($x$). The indirect transition (I) appears to be prominent compared to the direct one (A) in all the samples, as expected from TMD homobilayers. **b,** RC spectra measured at low temperature of isolated $Mo_xW_{(1\text{-}x)}Se_2$ alloys bilayers with different Mo concentrations ($x$). A and B exciton energies as a function of $x$ are displayed.

## SUPPLEMENTARY NOTE S3:. $Mo_xW_{(1-x)}Se_2/WSe_2$ HETEROSTRUCTURES MICROSCOPE IMAGES AND PL MAPS

In this section we present the optical characterization of the $Mo_xW_{(1-x)}Se_2/WSe_2$ heterobilayers at room and low temperature by means of microscope photoluminescence (PL) and bright field (BF) images and PL spatial maps. For each structure, the morphology of TMD monolayers and their optical behaviour in the heterojunction areas are highlighted in order to evidence the formation of inter-layer (IX) excitons. The low temperature PL color maps are built by measuring a PL spectrum for each point of the scanned area and then integrating the emission intensity in the desired spectral range. Further characterization details are described in the Methods section. The IX spectra showed in Fig.2b and the IX data used for Fig.2c of the main article are extracted from the following low temperature PL maps.

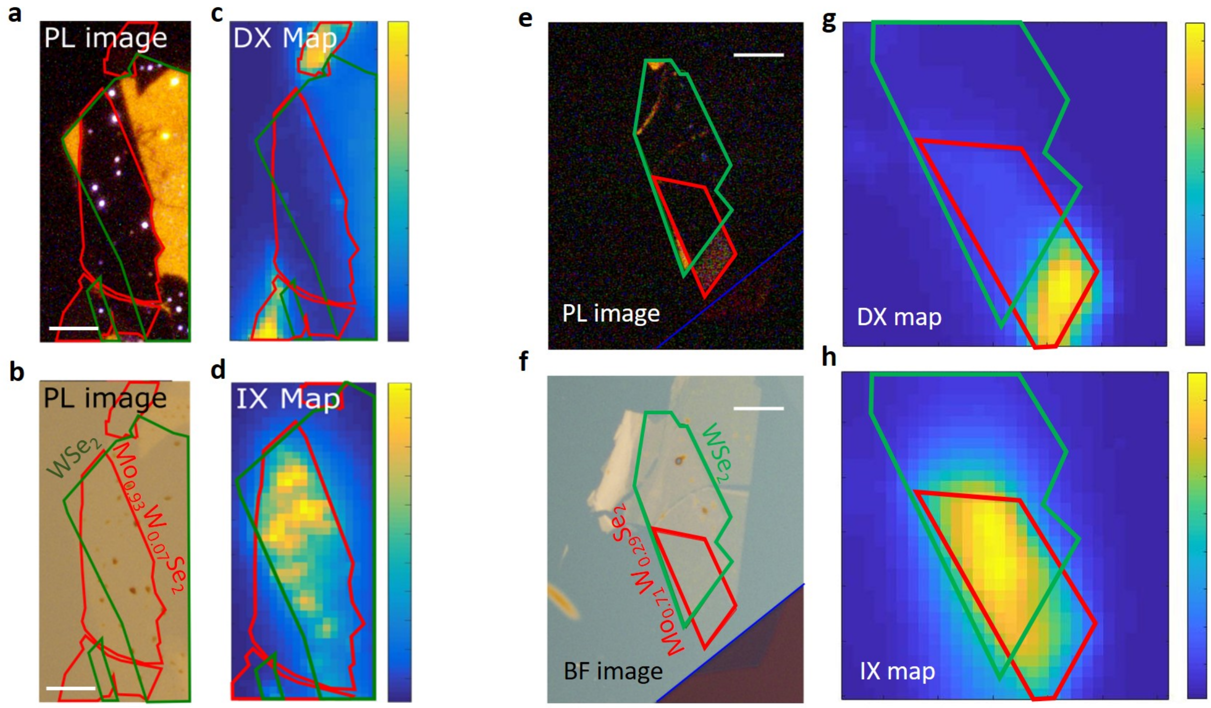


**Supplementary Figure S4.** **Microscope images and PL maps for $\mathbf{Mo_{0.93}W_{0.07}Se_2/WSe_2}$ and $\mathbf{Mo_{0.71}W_{0.29}Se_2/WSe_2}$ heterostructures.a,** PL microscope image of the $Mo_{0.93}W_{0.07}Se_2/WSe_2$ heterobilayer taken at room temperature. The quenching of PL signal in the heterobilayer region indicates a good electronic coupling and an efficient charge separation. The red line is the silhouette of the $Mo_{0.93}W_{0.07}Se_2$ flake while green solid line indicates the $WSe_2$ flake. The bare alloy flake is dark as expected considering its composition close to $MoSe_2$ **b,** BF image of the heterostructure taken at room temperature. **c,** Low temperature PL map of the heterostructure in the DX emission spectral region (1.45-1.7 eV energy range). The image looks complementary to the one shown in panel **a**. **d,** Low temperature PL map of the heterostructure in the IX emission spectral region (1.3-1.45 eV energy range). Bright PL is detected in correspondence of the heterobilayer and absent in the other regions. **e,** PL microscope image of the $Mo_{0.71}W_{0.29}Se_2/WSe_2$ heterobilayer taken at room temperature. The red line is the silhouette of the $Mo_{0.71}W_{0.29}Se_2$ flake while green solid line indicates the $WSe_2$ flake. The $WSe_2$ emission from the upper part of the flake is hidden by a thick alloy layer on top of it. **f,** BF image of the heterostructure taken at room temperature. **g,** Low temperature PL map of the heterostructure in the DX emission spectral region (1.43-1.78 eV energy range). **h,** Low temperature PL map of the heterostructure in the IX emission spectral region (1.24-1.475 eV energy range). Scale bars for (**a, b, e, f**), 10 $\mu$m.

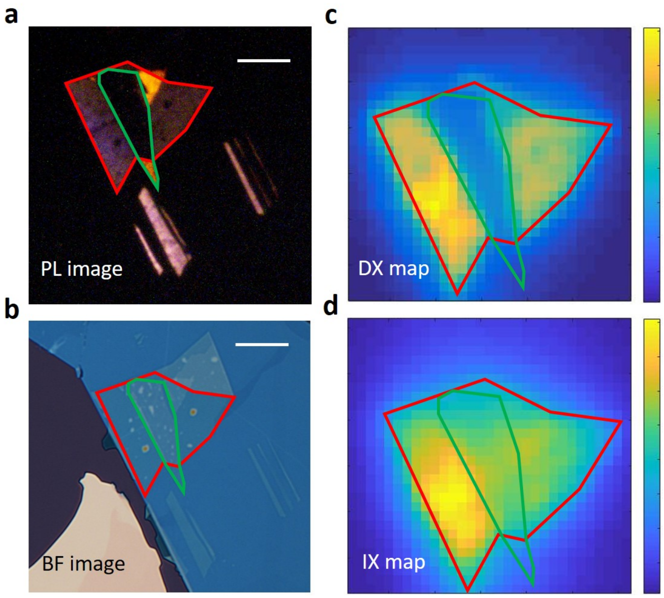


**Supplementary Figure S5**. **Microscope images and PL maps for $\mathbf{Mo_{0.64}W_{0.36}Se_2/WSe_2}$ heterostructure.a,** PL microscope image of the $Mo_{0.64}W_{0.36}Se_2/WSe_2$ heterobilayer taken at room temperature. The quenching of PL signal in the heterobilayer region indicates a good electronic coupling and an efficient charge separation. The red line is the silhouette of the $Mo_{0.64}W_{0.36}Se_2$ flake while green solid line indicates the $WSe_2$ flake. The bare alloy flake is dark as expected considering its composition close to $MoSe_2$ **b,** BF image of the heterostructure taken at room temperature. **c,** Low temperature PL map of the heterostructure in the DX emission spectral region (1.49-1.8 eV energy range). The image looks complementary to the one shown in panel **a**. **d,** Low temperature PL map of the heterostructure in the IX emission spectral region (1.305-1.49 eV energy range). Scale bars for (**a, b**), 10 $\mu$m.

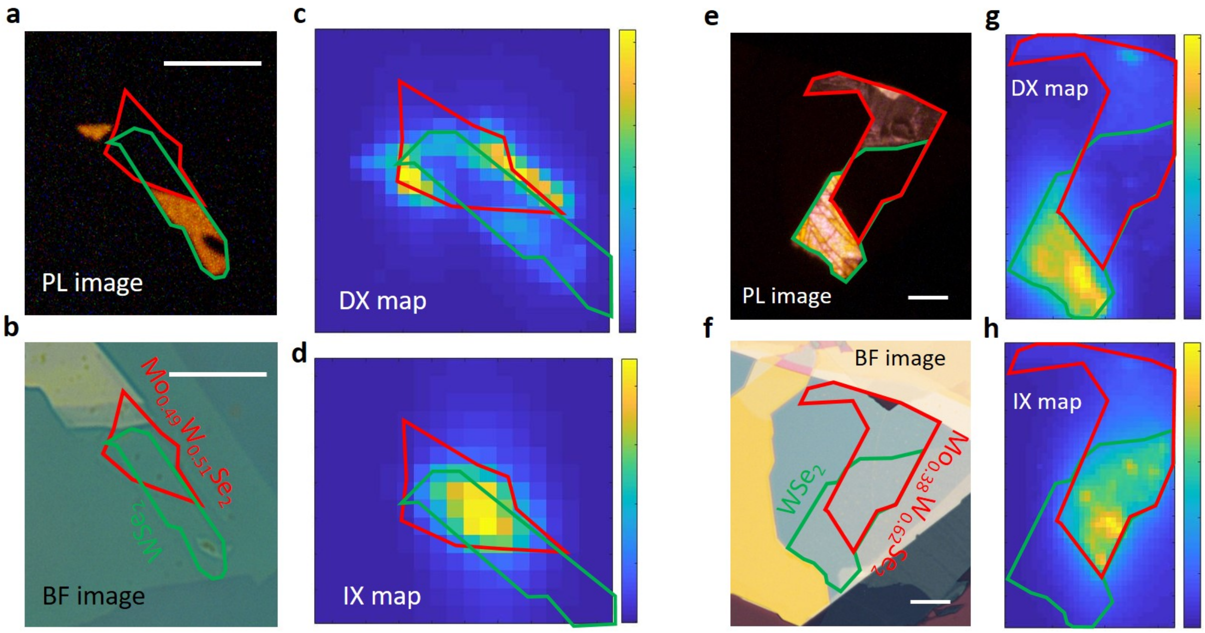


**Supplementary Figure S6**. **Microscope images and PL maps for $Mo_{0.49}W_{0.51}Se_2/WSe_2$ and $Mo_{0.38}W_{0.62}Se_2/WSe_2$ heterostructures.a,** PL microscope image of the $Mo_{0.49}W_{0.51}Se_2/WSe_2$ heterobilayer taken at room temperature. The quenching of PL signal in the heterobilayer region indicates a good electronic coupling and an efficient charge separation. The red line is the silhouette of the $Mo_{0.49}W_{0.51}Se_2$ flake while green solid line indicates the $WSe_2$ flake. The bare alloy flake is dark as expected considering its composition close to $MoSe_2$ **b,** BF image of the heterostructure taken at room temperature. **c,** Low temperature PL map of the heterostructure in the DX emission spectral region (1.52-1.92 eV energy range). The image looks complementary to the one shown in panel **a**. **d,** Low temperature PL map of the heterostructure in the IX emission spectral region (1.36-1.52 eV energy range). Bright PL is detected in correspondence of the heterobilayer and absent in the other regions. **e,** PL microscope image of the $Mo_{0.38}W_{0.62}Se_2/WSe_2$ heterobilayer taken at room temperature. The red line is the silhouette of the $Mo_{0.38}W_{0.62}Se_2$ flake while green solid line indicates the $WSe_2$ flake. Since the composition of the alloy is closer to $WSe_2$, the alloy emission intensity is comparable to $WSe_2$ both at room and low temperature. **f,** BF image of the heterostructure taken at room temperature. **g,** Low temperature PL map of the heterostructure in the DX emission spectral region (1.43-1.78 eV energy range). **h,** Low temperature PL map of the heterostructure in the IX emission spectral region (1.24-1.475 eV energy range). Scale bars for (**a, b, e, f**), 10 $\mu$m.

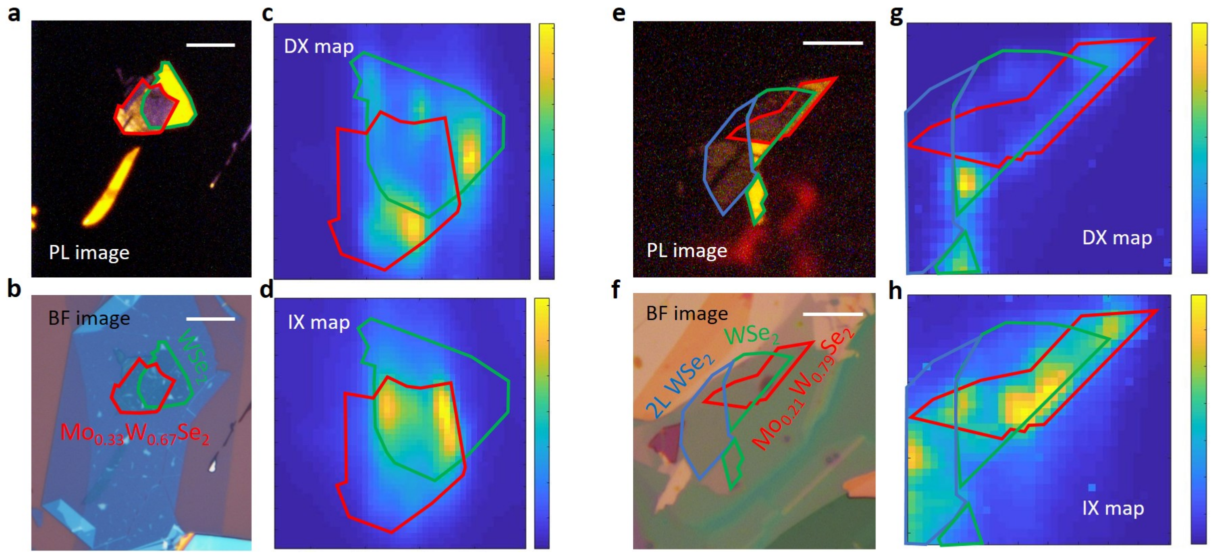


**Supplementary Figure S7**. **Microscope images and PL maps for $Mo_{0.33}W_{0.67}Se_2/WSe_2$ and $Mo_{0.21}W_{0.79}Se_2/WSe_2$ heterostructures.a,** PL microscope image of the $Mo_{0.33}W_{0.67}Se_2/WSe_2$ heterobilayer taken at room temperature. The quenching of PL signal in the heterobilayer region indicates a good electronic coupling and an efficient charge separation. The red line is the silhouette of the $Mo_{0.33}W_{0.67}Se_2$ flake while green solid line indicates the $WSe_2$ flake. The bare alloy flake is almost as bright as $WSe_2$, as expected considering its composition close to the latter. **b,** BF image of the heterostructure taken at room temperature. **c,** Low temperature PL map of the heterostructure in the DX emission spectral region (1.55-1.75 eV energy range). **d,** Low temperature PL map of the heterostructure in the IX emission spectral region (1.41-1.55 eV energy range). Bright PL is detected in correspondence of the heterobilayer and absent in the other regions. **e,** PL microscope image of the $Mo_{0.21}W_{0.79}Se_2/WSe_2$ heterobilayer taken at room temperature. The red line is the silhouette of the $Mo_{0.21}W_{0.79}Se_2$ flake while green solid line indicates the $WSe_2$ flake and blue solid line refers to a bilayer of $WSe_2$. **f,** BF image of the heterostructure taken at room temperature. **g,** Low temperature PL map of the heterostructure in the DX emission spectral region (1.42-1.75 eV energy range). **h,** Low temperature PL map of the heterostructure in the IX emission spectral region (1.24-1.42 eV energy range). The PL intensity in the heterobilayer area is comparable to the one emitted by the homobilayer. Scale bars for (**a, b, e, f**), 10 $\mu$m.

## SUPPLEMENTARY NOTE S4:. PEAK ANALYSIS OF IX PL SPECTRA IN $Mo_xW_{(1-x)}Se_2$ /$WSe_2$ HBLS

The structured PL spectra of IXs measured in the $WSe_2$/alloy HBLs with different Mo concentration evidence multiple peaks (Fig.2b of the main text). A detailed analysis of such spectra is displayed in Figure S8 where each experimental plot is fitted with three or four Gaussian curves. The peak positions extracted from the fitting are plotted as a function of the alloy Mo content in Fig.S8i as squares, triangles and circles, where the less dominant peaks are indicated by empty diamonds. The highest IX peak energies extracted from this analysis are included as blue squares in Fig.2c of the main text. All the IX peaks clearly blue-shift as the Mo concentration $x$ in the alloy decreases, reaching asymptotically an energy of about 1.5 eV (see the main text for our full explanation).

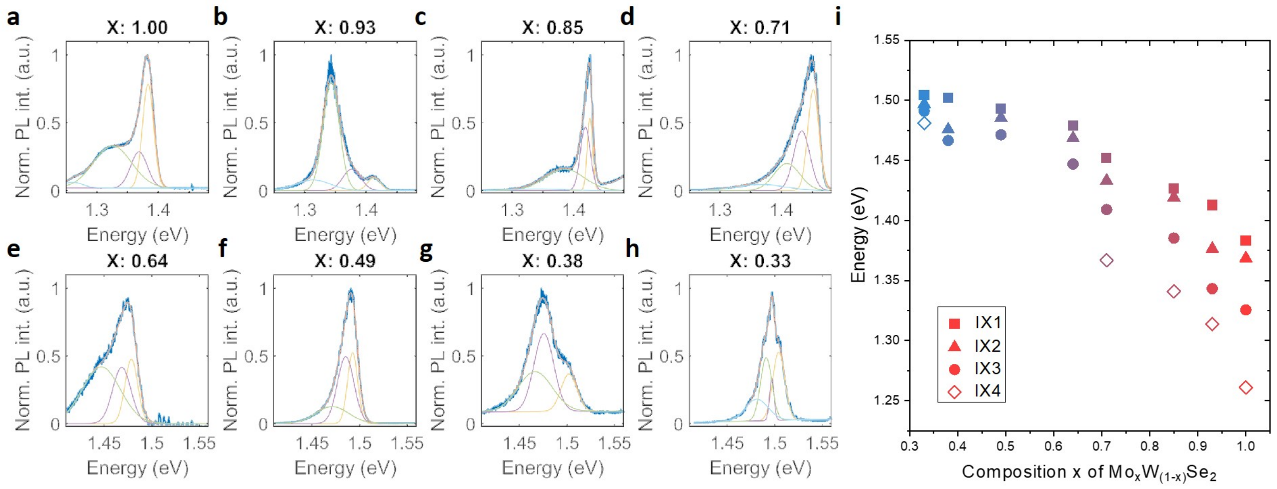


**Supplementary Figure S8**. **IXs PL spectra analysis in alloys/$WSe_2$ HBLs. a, b, c, d, e, f, g, h,** Normalized PL spectra of the $Mo_xW_{(1-x)}Se_2$/$WSe_2$ HBLs measured at 10K for different alloys compositions $x$ (blue lines), fitted by three or four Gaussian peak functions. The fit sum is shown with an orange line. **i,** Peak positions extracted from the fits of the alloy/$WSe_2$ IX PL spectra as a function of Mo composition x in the alloy layer. The symbols IX1, IX2, IX3, IX4 refer to the four different IX peaks found at decreasing energies (extracted respectively from the yellow, purple, green and sky blue lines in the first panels). IX1 energies are also shown as blue squares in Fig. 2c of the main text.

Even for a non-alloyed $WSe_2$/$MoSe_2$ HBL, the exact origin of these peaks is still under debate, due to its complex electronic band structure. As clearly pointed out in [1], depending on the different experiments and theoretical calculations, the main PL features can be attributed to 1) a mix of momentum direct (K→K) and momentum-indirect (K→Q) interlayer excitons, the former being at higher energy, as shown by temperature-dependent behavior of the exciton lifetimes at the different IX wavelengths; [2, 3] 2) only to momentum-indirect K→Q excitons, with an

energy separation due to the spin–orbit splitting of the conduction band valley at the Q point, demonstrated by the observed opposite circular polarization behaviour;[4] 3) a singlet–triplet pair of momentum-direct excitons at the K and K' points, as shown by the IX PL measurements applying an external magnetic fields;[5–8] and 4) a combination of neutral and charged spatially indirect excitons.[9] In our experiments we might measure signals from IXs of all those different natures. Very recently, crucial experiments of differential reflectivity under a modulated electric field unveiled the exact dipole moment and spectral position of the momentum-direct IXs, observed at higher energy compared to the momentum-indirect ones. [10] The latter has been found more visible in the PL spectra at low excitation powers, while the momentum-direct IX states have been efficiently populated by increasing the temperature or the excitation density, corroborating the explanation 1).

## SUPPLEMENTARY NOTE S5:. $Mo_xW_{(1-x)}Se_2/WSe_2$ HETEROSTRUCTURES PL INTENSITIES

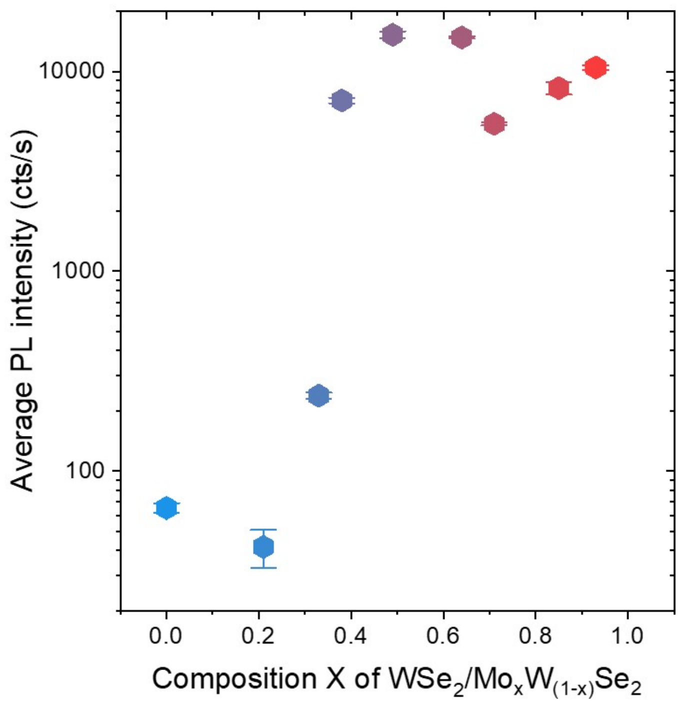


**Supplementary Figure S9**. **$Mo_xW_{(1-x)}Se_2/WSe_2$ heterostructures PL intensities.** Average PL intensity of $Mo_xW_{(1-x)}Se_2/WSe_2$ heterostructures extracted from the low temperature PL maps of Fig.SI 4-7. The data are mediated among an average of up to 60 different points chosen within the heterobilayer areas of each structure. The error bars depict the calculated statistical variation from the average value. The mean intensity drops of about 2 orders of magnitude as the alloy composition approaches the $WSe_2$ one.

## SUPPLEMENTARY NOTE S6:. STUDY ON $\mathbf{Mo}_x\mathbf{W}_{(1-x)}\mathbf{Se}_2$/$\mathbf{MoSe}_2$ HETEROSTRUCTURES

As shown for $Mo_xW_{(1-x)}Se_2$/$\mathbf{WSe_2}$ HBLs in the main text, in this section we present the optical characterization of the $Mo_xW_{(1-x)}Se_2$/$\mathbf{MoSe_2}$ heterobilayers. Specifically, for each sample we recorded microscope photoluminescence (PL) and bright field (BF) images at room temperature and we measured PL spatial maps at low temperature. From the latter we also extracted the PL spectra of the IX transitions appearing in the heterobilayers.

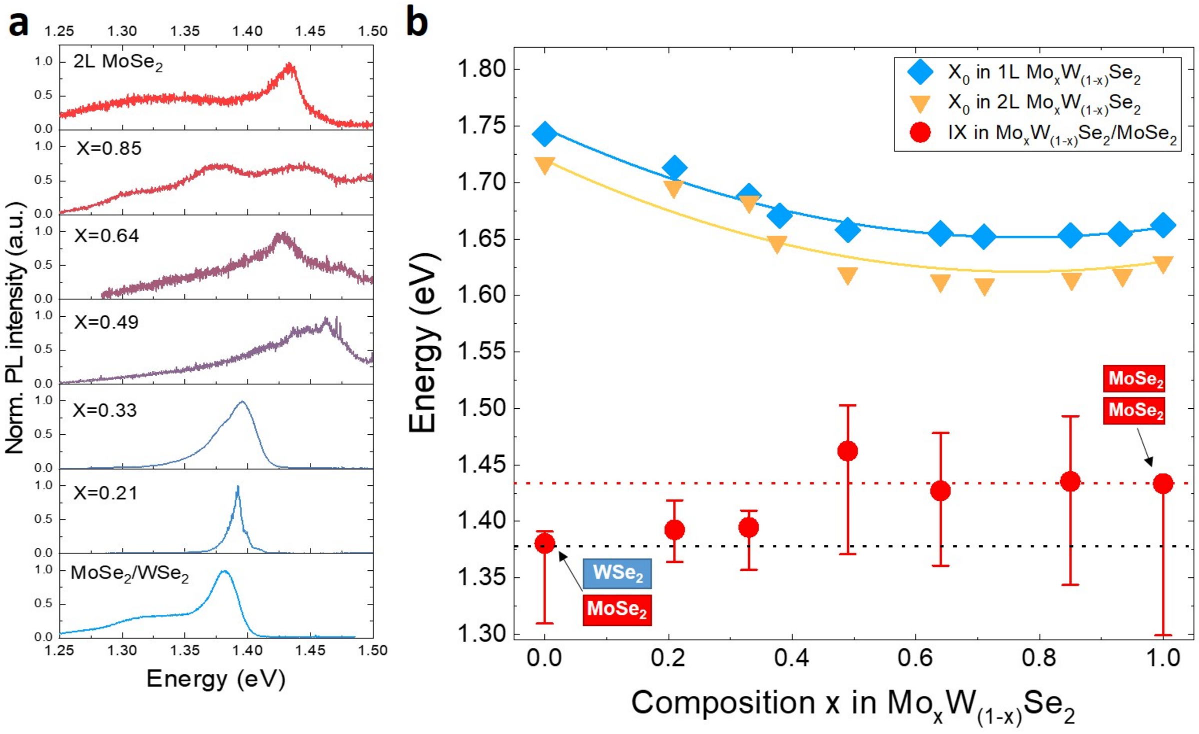


**Supplementary Figure S10**. **IX emission spectra for $\mathbf{Mo}_x\mathbf{W}_{(1-x)}\mathbf{Se}_2$/$\mathbf{MoSe}_2$ heterostructures.** **a** Normalized PL spectra of the $Mo_xW_{(1-x)}Se_2$/$MoSe_2$ heterostructures measured at 4K for different alloys compositions. **b** Peak position of the highest energy IX peak in the alloy/$MoSe_2$ (red circles) HBLs as a function of Mo composition $x$ in the alloy layer, together with the neutral exciton peak position of the alloy monolayers (sky blue diamonds) and bilayers (yellow triangles). The error bars depict the spread in energy of multiple indirect transitions peaks, calculated as the standard deviation from the average PL wavelength. Sky blue and orange solid lines are parabolic fits of the DX peak energy in isolated alloy monolayers and bilayer respectively. The dashed black (red) horizontal line refers to the IX energy in $MoSe_2$/$WSe_2$ HBLs ($MoSe_2$ homobilayers).

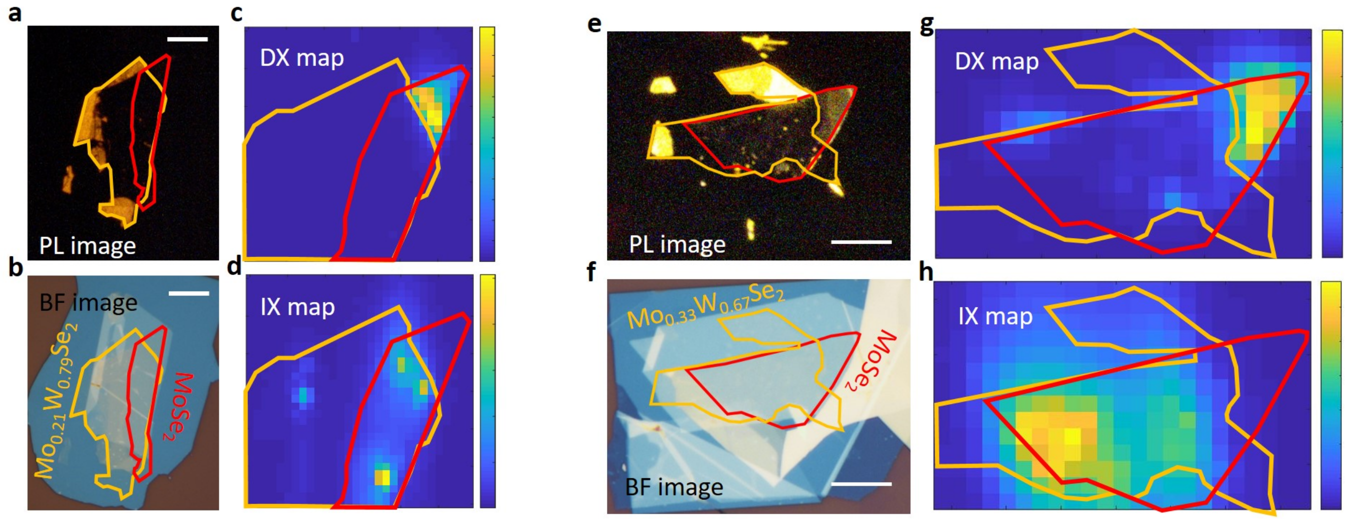


**Supplementary Figure S11**. **Microscope images and PL maps for $Mo_{0.33}W_{0.67}Se_2/MoSe_2$ and $Mo_{0.21}W_{0.79}Se_2/MoSe_2$ heterostructures.a,** PL microscope image of the $Mo_{0.21}W_{0.79}Se_2/MoSe_2$ heterobilayer taken at room temperature. The quenching of PL signal in the heterobilayer region indicates a good electronic coupling and an efficient charge separation. The red line is the silhouette of the $MoSe_2$ flake while the dark yellow solid line indicates the $Mo_{0.21}W_{0.79}Se_2$ flake. The bare alloy flake is bright at RT, as expected considering its composition close to $WSe_2$. **b,** BF image of the heterostructure taken at room temperature. **c,** Low temperature PL map of the heterostructure in the DX emission spectral region (1.55-1.77 eV energy range). **d,** Low temperature PL map of the heterostructure in the IX emission spectral region (1.3-1.55 eV energy range). Bright PL is detected in the heterobilayer area and absent in the other regions. Some brighter spots appear, most probably where the coupling between the two layers is higher. **e,** PL microscope image of the $Mo_{0.33}W_{0.67}Se_2/MoSe_2$ heterobilayer taken at room temperature. The red line is the silhouette of the $MoSe_2$ flake while the dark yellow solid line indicates the $Mo_{0.33}W_{0.67}Se_2$ flake. **f,** BF image of the heterostructure taken at room temperature. **g,** Low temperature PL map of the heterostructure in the DX emission spectral region (1.43-1.65 eV energy range). **h,** Low temperature PL map of the heterostructure in the IX emission spectral region (1.24-1.43 eV energy range). Bright PL is detected in correspondence of the heterobilayer and absent in the other regions. Scale bars for (**a, b, e, f**), 10 $\mu$m.

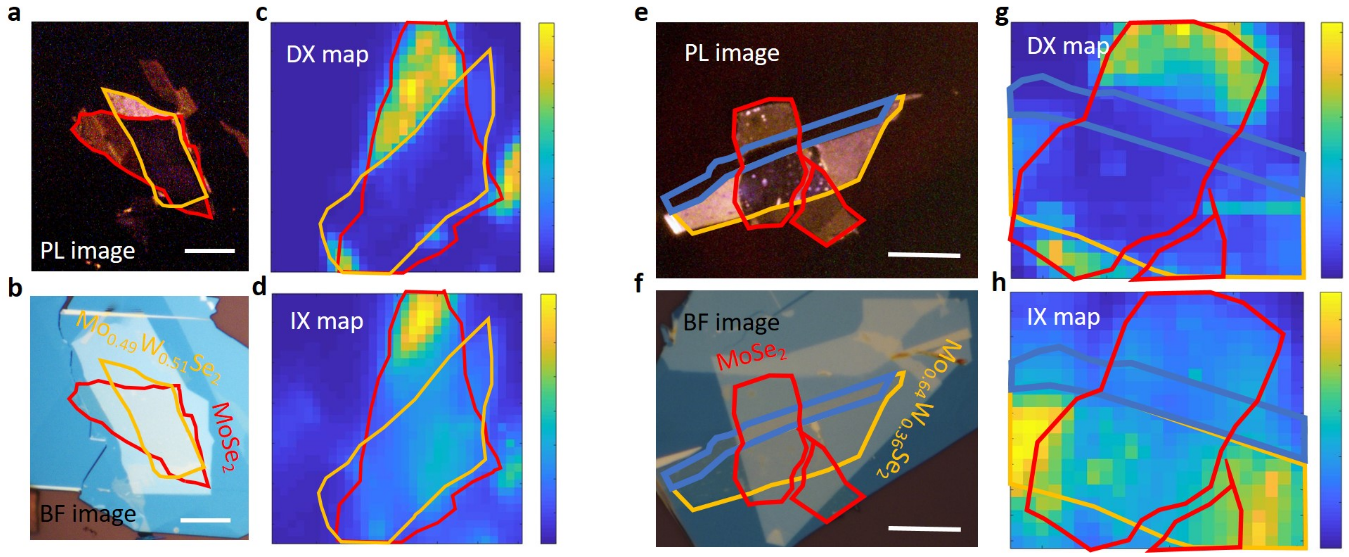


**Supplementary Figure S12**. **Microscope images and PL maps for $Mo_{0.49}W_{0.51}Se_2/MoSe_2$ and $Mo_{0.64}W_{0.36}Se_2/MoSe_2$ heterostructures.a,** PL microscope image of the $Mo_{0.49}W_{0.51}Se_2/MoSe_2$ heterobilayer taken at room temperature. The quenching of PL signal in the heterobilayer region indicates a good electronic coupling and an efficient charge separation. The red line is the silhouette of the $MoSe_2$ flake while the dark yellow solid line indicates the $Mo_{0.49}W_{0.51}Se_2$ flake. **b,** BF image of the heterostructure taken at room temperature. **c,** Low temperature PL map of the heterostructure in the DX emission spectral region (1.53-1.65 eV energy range). Bright PL is detected only outside the heterobilayer area. **d,** Low temperature PL map of the heterostructure in the IX emission spectral region (1.36-1.53 eV energy range). PL emission from the heterobilayer area is visible, despite being less bright than some zones of the $MoSe_2$ flake not covered by the top hBN. **e,** PL microscope image of the $Mo_{0.64}W_{0.36}Se_2/MoSe_2$ heterobilayer taken at room temperature. The red line is the silhouette of the $MoSe_2$ flake while the dark yellow solid line indicates the $Mo_{0.64}W_{0.36}Se_2$ flake. The blue line refers to a thick part of the alloy flake. **f,** BF image of the heterostructure taken at room temperature. **g,** Low temperature PL map of the heterostructure in the DX emission spectral region (1.53-1.65 eV energy range). Bright PL is detected only outside the heterobilayer area. **h,** Low temperature PL map of the heterostructure in the IX emission spectral region (1.36-1.53 eV energy range). PL emission from the heterobilayer area is visible, despite being less bright than some zones of the bare alloy monolayer, most probably due to the IX transition becoming momentum-indirect in this heterobilayer (see main text). Scale bars for (**a, b, e, f**), 10 $\mu$m.

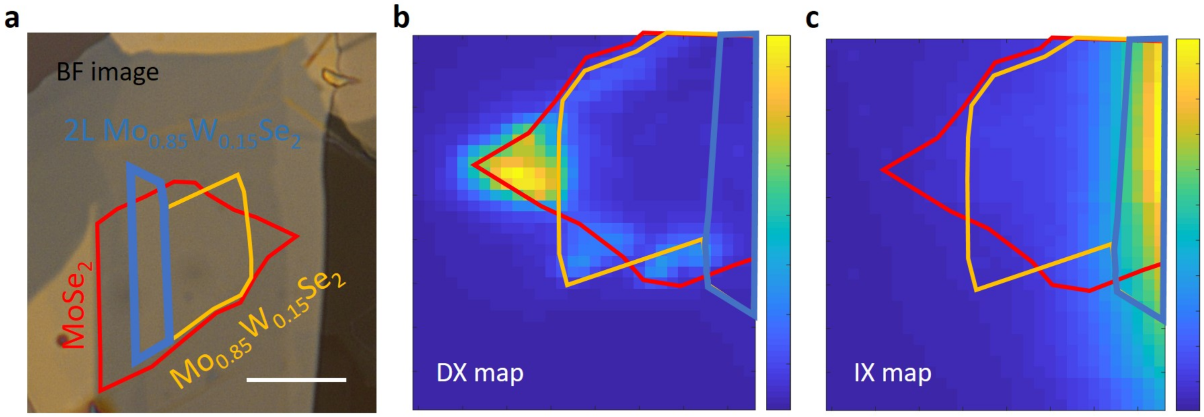


**Supplementary Figure S13**. **Microscope images and PL maps for a $Mo_{0.85}W_{0.15}Se_2$/$MoSe_2$ heterostructure.a,** BF microscope image of the $Mo_{0.85}W_{0.15}Se_2$/$MoSe_2$ heterobilayer taken at room temperature. The red line is the silhouette of the $MoSe_2$ flake while the dark yellow solid line indicates the $Mo_{0.49}W_{0.51}Se_2$ flake. The blue line refers to the alloy homobilayer. The PL microscope image (not shown) for this structure is completely dark because of the presence of $MoSe_2$ and $Mo_{0.85}W_{0.15}Se_2$, being both dark at room temperature. **b,** Low temperature PL map of the heterostructure in the DX emission spectral region (1.51-1.67 eV energy range). Bright PL is detected only outside the heterobilayer area. **c,** Low temperature PL map of the heterostructure in the IX emission spectral region (1.38-1.51 eV energy range). In this case the IX PL emission is mostly coming from the overlapping area between the $MoSe_2$ and the alloy bilayer, since the exciton transitions in the heterobilayer area are momentum-indirect. Scale bars for (**a, b**), 10 $\mu$m.

## SUPPLEMENTARY NOTE S7:. CONDUCTION AND VALENCE BANDS OFFSETS

In this section, we describe two theoretical approximations to the $WSe_2/Mo_xW_{(1-x)}Se_2$ HS conduction- and valence band offsets; one that neglects hybridisation between the constituting $WSe_2$ and alloy layers, and a second one that includes it.

In the first approximation, $x$-dependent conduction- and valence band offsets $\Delta CB(x)$ and $\Delta VB(x)$ can be estimated by simple interpolation between the to limiting cases of a perfect $WSe_2/MoSe_2$ heterostructure ($x = 1$), and a perfect $WSe_2$ bilayer ($x = 0$). In the former case, the band offsets are

$$\begin{aligned} \Delta \mathrm{CB} =& E_g^{\mathrm{WSe_2}} - E_g^{\mathrm{WSe_2/MoSe_2}} \approx E_{DX}^{\mathrm{WSe_2}} - E_{\mathrm{IX}}^{\mathrm{WSe_2/MoSe_2}}, \\ \Delta \mathrm{VB} =& E_g^{\mathrm{MoSe_2}} - E_g^{\mathrm{WSe_2/MoSe_2}} \approx E_{DX}^{\mathrm{MoSe_2}} - E_{\mathrm{IX}}^{\mathrm{WSe_2/MoSe_2}}, \end{aligned} \tag{S1}$$

where $E_g^{\mathrm{WSe_2}}$ and $E_g^{\mathrm{MoSe_2}}$ represent the intralayer band gaps of the corresponding layers, and $E_g^{\mathrm{WSe_2/MoSe_2}}$ is the HS band gap. In Eq. (S1), we have approximated these gap energies by the corresponding direct- and indirect exciton energies, thus neglecting the exciton binding energies and incurring an error $\sim 10\,\mathrm{meV}$. Both band offsets vanish in the case of $x = 0$, and we may interpolate between the two cases using the parameters obtained for the direct exciton in the alloy, assuming a linear interpolation for the valence band offset, and assigning the bowing parameter exclusively to the conduction band offset. This is justified based on recent reports[11] on the orbital compositions of the $WSe_2$ and $MoSe_2$ $K$-point band edges, showing that, whereas the valence bands of the two materials share a common orbital composition ($d_{xy}$ and $d_{x^2-y^2}$), the conduction bands are formed by different orbital mixtures. This suggests a simple linear interpolation in the former case, and a non linear one in the latter. The corresponding interpolating formulas are

$$\begin{aligned} \Delta E1(x) =& x\Delta \mathrm{CB} + x(1-x)b, \\ \Delta E2(x) =& x\Delta \mathrm{VB}, \end{aligned} \tag{S2}$$

with $b = 0.16\,\mathrm{eV}$ is the bowing parameter reported in Fig. **S2** for the A exciton in the alloy. The resulting curves are shown with dashed lines in Fig. **S14** and in Main Text Fig. 4a, where it is clear that this non-hybridised approximation is valid only for $x \to 1$, whereas for $x \lesssim 0.6$ it fails to reproduce the experimental results. As discussed in the main text, we attribute this discrepancy to a transition from a direct band gap at the $K$ point for HSs with $0.6 \lesssim x \leq 1$, to an indirect band gap for $0 \leq x \lesssim 0.6$.

To further examine this direct-to-indirect transition of the HS band gap, we introduce a simple theoretical model with no free parameters for interlayer band hybridisation at three relevant points in the Brillouin zone (BZ): $K$

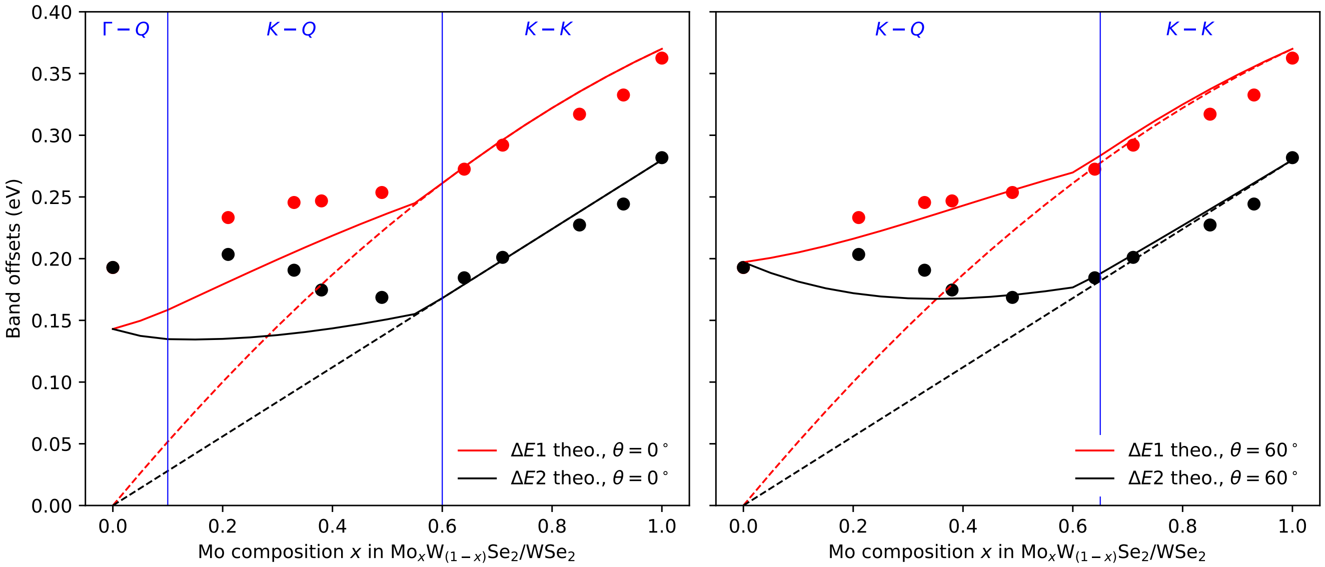


**Supplementary Figure S14**. Comparison between the experimentally determined band offsets, and the theoretical predictions obtained assuming 0° (left) and 60° (right) HSs. For each range of $x$ values, the BZ momenta of the lowest energy optical transition (hole–electron) giving rise to the indirect exciton is indicated in blue. In both panels, the red (black) circles are the experimental values of $\Delta E1$ ($\Delta E2$), whereas the red (black) dashed lines are the corresponding theoretical values in the non hybridised approximation of Eq. (S2).

(conduction and valence bands), $Q$ (conduction band) and $\Gamma$ (valence band). Due to momentum conservation, the Hamiltonians at all three BZ points are mutually independent. Moreover, in each case we neglect hybridisation between the conduction and valence bands of opposite layers, as justified by the small tunnelling energy ($\sim 0.01\,\mathrm{eV}$) to band gap ($\sim 1\,\mathrm{eV}$) ratio[12–14]. Our computations consider both possible HS alignments of our samples, $\theta \approx 0°$ and 60°, and assume either full commensurability or domain formation via in-plain relaxation between the $WSe_2$ and alloy layers[15, 16]. The corresponding Hamiltonians take the form

$$H_K^{\mathrm{CB}}(\theta) = \begin{pmatrix} E_{\mathrm{WSe_2}}^{\mathrm{CB}}(\theta) & t_K^{\mathrm{CB}}(\theta) \\ t_K^{\mathrm{CB}\,*}(\theta) & E_{\mathrm{alloy}}^{\mathrm{CB}}(\theta) \end{pmatrix}, \quad H_K^{\mathrm{VB}}(\theta) = \begin{pmatrix} E_{\mathrm{WSe_2}}^{\mathrm{VB}}(\theta) & t_K^{\mathrm{VB}}(\theta) \\ t_K^{\mathrm{VB}\,*}(\theta) & E_{\mathrm{alloy}}^{\mathrm{VB}}(\theta) \end{pmatrix},$$
$$H_Q^{\mathrm{CB}}(\theta) = \begin{pmatrix} E_{\mathrm{WSe_2}}^{\mathrm{CB}}(\theta) + \delta_{\mathrm{WSe_2}}^{Q} & t_Q(\theta) \\ t_Q^*(\theta) & E_{\mathrm{alloy}}^{\mathrm{CB}}(\theta) + \delta_{\mathrm{alloy}}^{Q} \end{pmatrix}, \quad H_\Gamma^{\mathrm{VB}}(\theta) = \begin{pmatrix} E_{\mathrm{WSe_2}}^{\mathrm{CB}}(\theta) - \delta_{\mathrm{WSe_2}}^{\Gamma} & t_\Gamma \\ t_\Gamma^* & E_{\mathrm{alloy}}^{\mathrm{CB}}(\theta) - \delta_{\mathrm{alloy}}^{\Gamma} \end{pmatrix}. \tag{S3}$$

Here, $E_{\mathrm{WSe_2}}^{\alpha}(\theta)$ and $E_{\mathrm{alloy}}^{\alpha}(\theta)$ are the monolayer conduction ($\alpha$ = CB) and valence ($\alpha$ = VB) band edge energies of the $WSe_2$ and alloy layers, at the $K$ point; $\delta_{\mathrm{WSe_2}}^{Q}$ and $\delta_{\mathrm{alloy}}^{Q}$ are the energy offsets between the $K$ and $Q$ point conduction-band edges of the $WSe_2$ and alloy monolayers, respectively; and $\delta_{\mathrm{WSe_2}}^{\Gamma}$ and $\delta_{\mathrm{alloy}}^{\Gamma}$ have analogous definitions

with respect to the monolayer valence bands. In all cases, the off-diagonal parameters are angle-dependent interlayer tunnelling energies. We have taken all tunnelling energies and energy offsets from Ref. [14], where they have been extracted from a combination of symmetry analysis and density functional theory calculations, and compiled them in Table S2.

As before, we set our energy reference at the HS valence-band edge, so that $E^{\mathrm{VB}}_{\mathrm{WSe_2}}(0°) = 0$. For $\theta = 0°$, we may identify the monolayer band gaps with the HS intralayer exciton energies, e.g., $E^{\mathrm{CB}}_{\mathrm{WSe_2}}(0°) \approx E^{\mathrm{WSe_2}}_{DX} = 1.743\,\mathrm{eV}$, because intralayer hybridisation vanishes at the $K$ point for 0° structures (Table S2). This also gives us $E^{\mathrm{VB}}_{\mathrm{MoSe_2}}(0°) = E^{\mathrm{VB}}_{\mathrm{WSe_2}} - \Delta E2^*$ and $E^{\mathrm{CB}}_{\mathrm{MoSe_2}}(0°) = E^{\mathrm{CB}}_{\mathrm{WSe_2}} - \Delta E1^*$, where $\Delta E1^*$ and $\Delta E2^*$ are experimental values obtained form the $x = 1$ samples. Then, all alloy band energies are obtained by interpolation between the $WSe_2$ and $MoSe_2$ values, assigning the measured bowing parameter to the $x$ dependence of the conduction band, as discussed above.

Once all parameters have been set for each Mo concentration $x$, we diagonalise all Hamiltonians to find the HS conduction- and valence band edges, and their location in the BZ. This determines the HS band gap $E^{\mathrm{HS}}_g$, and approximately the indirect exciton energy $E_{\mathrm{IX}}$, whereas the intralayer direct excitons in both the $WSe_2$ and alloy layers remain at the $K$ point, and approximately non hybridised. This allows us to estimate the conduction- and valence band offsets as

$$\Delta E1(x) \approx E^{\mathrm{WSe_2}}_{\mathrm{DX}} - E^{\mathrm{HS}}_g(x), \quad \Delta E2(x) \approx E^{\mathrm{alloy}}_{\mathrm{DX}}(x) - E^{\mathrm{HS}}_g(x). \tag{S4}$$

The results for $\theta = 0°$, presented in the left panel of Fig. **S14**, show poor agreement with the experimental data, undershooting the $x = 0$ band offset values by about 50 meV.

By contrast to the 0° case, $K$-point interlayer hybridisation is finite for 60° structures (Table S2), such that the $WSe_2$ ($MoSe_2$) $K$-point monolayer band edge energies will differ from those measured in the HS by an upward (downward) shift of magnitude

$$-\frac{\Delta E1^*}{2} + \sqrt{\left(\frac{\Delta E1^*}{2}\right)^2 + |t^{\mathrm{CB}}_K(60°)|^2}$$

for the conduction band, and

$$-\frac{\Delta E2^*}{2} + \sqrt{\left(\frac{\Delta E2^*}{2}\right)^2 + |t^{\mathrm{VB}}_K(60°)|^2}$$

for the valence band. Taking these corrections into account and using Eq. (S4), we obtain the $\Delta E1$ and $\Delta E2$ curves shown in the right panel of Fig. **S14**, which are in good agreement with the experimental data throughout the whole range of alloy concentrations. It must be pointed out that, for $x \to 1$, the good match between the calculations and

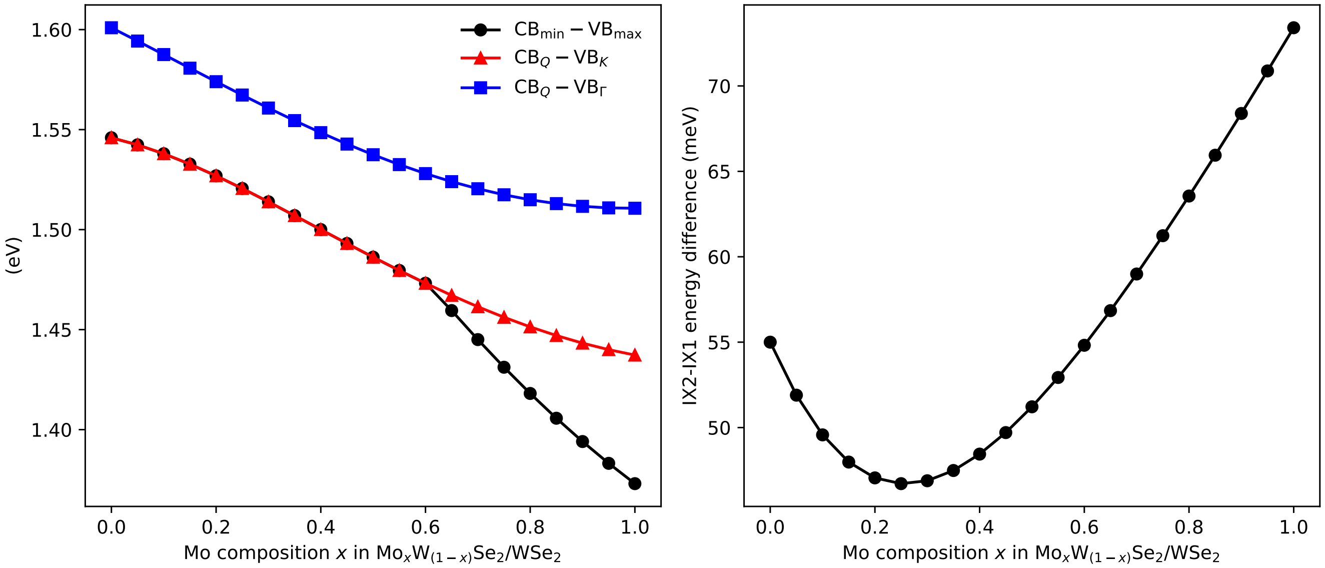


**Supplementary Figure S15**. (Left) Optical transition energies between the CB at $Q$ and the VB at $K$ ($K-Q$), between the CB at $Q$ and the VB at $\Gamma$ ($\Gamma - Q$), and between the overal CB minimum and VB maximum, as functions of Mo concentration $x$, predicted by the hybridisation models (S3). (Right) Energy difference between the higher-energy ($\Gamma - Q$) and lower-energy ($K - Q$) transitions, proposed to explain the presence of to IX PL peaks, IX1 and IX2.

the experimental data is by construction of the theoretical model. As a consequence, both the 0° and 60° calculations match the experiment for $0.65 < x \leq 1$. However, this is not the case for $x \to 0$, where only the 60° model gives an excellent match to the experimental data. This suggests that, at least for $x < 0.65$, the measured samples are H-stacked 60° HSs.

In addition to determining the band offsets, the above calculation reveals the BZ distribution of the HS band gap, and thus of the optical transition related to the indirect exciton peak. The numerical results show that the HS valence-band edge remains at the $K$ point throughout the range of Mo concentrations $x$, whereas the HS conduction-band edge changes from the $K$ point for $0.65 < x \leq 1$ to the $Q$ point for $0 \leq x < 0.65$, resulting in a direct-to-indirect gap transition at $x = 0.65$. This is indicated in Fig. **S14**.

Finally, Fig. **S15** shows a comparison between the $K - Q$ and $\Gamma - Q$ optical transition energies, as functions of the Mo concentration $x$, according to the hybridisation model (S3). The left panel shows that the minimum offset between the two transitions occurs somewhere between $x = 0.2$ and $x = 0.3$. As this offset is minimised, so is the thermal suppression of the $\Gamma - Q$ transition in PL due to its higher energy, making it possible for a PL peak associated to this transition to appear about 45 to 55 meV above the IX1 signature. This is consistent with our experimental

observation of the IX2 PL peak for the $x = 0.21$ sample.

| | $\theta \approx 0^\circ$ | $\theta \approx 60^\circ$ | | $\theta \approx 0^\circ$ | $\theta \approx 60^\circ$ |
|---|---|---|---|---|---|
| $E_{\mathrm{WSe_2}}^{\mathrm{VB}}$ | 0 | $-0.012$ | $\delta_{\Gamma}^{\mathrm{WSe_2}}$ | 0.620 | |
| $E_{\mathrm{WSe_2}}^{\mathrm{CB}}$ | 1.743 | 1.744 | $\delta_{\Gamma}^{\mathrm{MoSe_2}}$ | 0.480 | |
| $E_{\mathrm{MoSe_2}}^{\mathrm{VB}}$ | $-0.280$ | $-0.292$ | $\lvert t_K^{\mathrm{CB}} \rvert$ | 0 | 0.015 |
| $E_{\mathrm{MoSe_2}}^{\mathrm{CB}}$ | 1.373 | 1.372 | $\lvert t_K^{\mathrm{VB}} \rvert$ | 0 | 0.060 |
| $\delta_Q^{\mathrm{WSe_2}}$ | 0.030 | | $\lvert t_Q \rvert$ | 0.168 | 0.180 |
| $\delta_Q^{\mathrm{MoSe_2}}$ | 0.160 | | $\lvert t_\Gamma \rvert$ | 0.625 | |

TABLE S2. Theoretical model parameters. All band-edge energies were extracted from the measured exciton energies, neglecting binding energies, whereas all hybridisation parameters were taken from Ref. [14]. All values given in eV.

## SUPPLEMENTARY NOTE S8:. $Mo_xW_{(1-x)}Se_2/WSe_2$ HETEROSTRUCTURES PL SATURATION

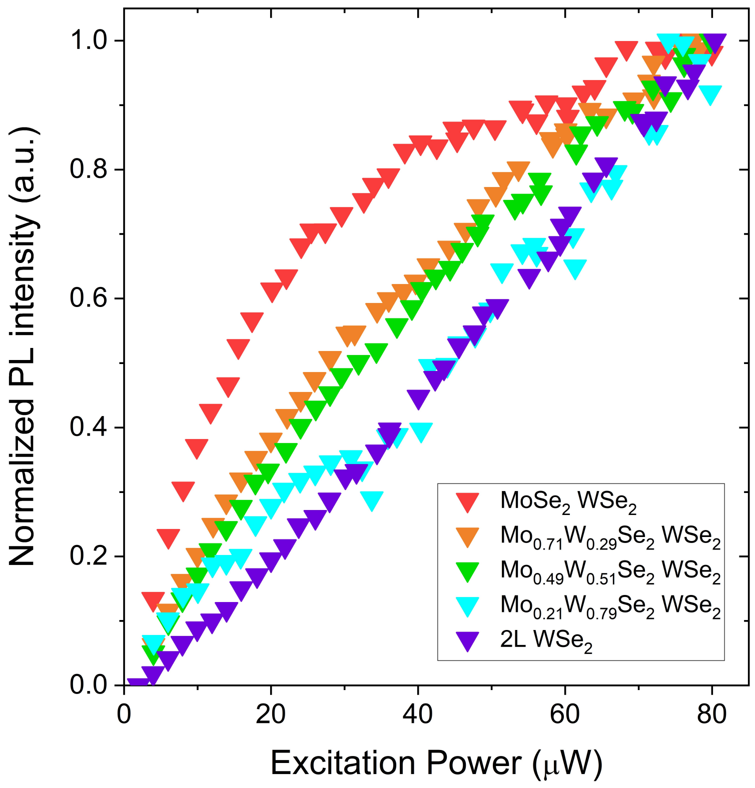


**Supplementary Figure S16**. **PL intensity saturation of IXs in $Mo_xW_{(1-x)}Se_2/WSe_2$ heterobilayers.** Normalized PL intensity versus excitation power measured at the IX peak wavelength in different $Mo_xW_{(1-x)}Se_2/WSe_2$ HSs. In the $MoSe_2/WSe_2$ sample, IX emission clearly exhibits a non-linear behaviour, which becomes less pronounced when the alloy composition gets close to $WSe_2$, tending towards a linear trend. For dipolar inter-layer excitons, the PL intensity saturate above a certain excitation power threshold, due to enhanced exciton-exciton annihilation processes or Auger non-radiative recombinations. This effect becomes less and less pronounced approaching the homobilayer configuration, when the IX dipoles lose their out-of-plane preferential orientation and their lifetime strongly decreases (see Fig.3a,b in the main text). All the samples have been excited by a 660nm CW laser.

[1] R. Gillen, Interlayer excitonic spectra of vertically stacked mose2/wse2 heterobilayers, physica status solidi (b) **258**, 2000614 (2021).

[2] P. Rivera, J. R. Schaibley, A. M. Jones, J. S. Ross, S. Wu, G. Aivazian, P. Klement, K. Seyler, G. Clark, N. J. Ghimire, *et al.*, Observation of long-lived interlayer excitons in monolayer mose2–wse2 heterostructures, Nature communications **6**, 1 (2015).

[3] B. Miller, A. Steinhoff, B. Pano, J. Klein, F. Jahnke, A. Holleitner, and U. Wurstbauer, Long-lived direct and indirect interlayer excitons in van der waals heterostructures, Nano letters **17**, 5229 (2017).

[4] A. T. Hanbicki, H.-J. Chuang, M. R. Rosenberger, C. S. Hellberg, S. V. Sivaram, K. M. McCreary, I. I. Mazin, and B. T. Jonker, Double indirect interlayer exciton in a mose2/wse2 van der waals heterostructure, ACS nano **12**, 4719 (2018).

[5] M. Förg, A. S. Baimuratov, S. Y. Kruchinin, I. A. Vovk, J. Scherzer, J. Förste, V. Funk, K. Watanabe, T. Taniguchi, and A. Högele, Moiré excitons in mose2-wse2 heterobilayers and heterotrilayers, Nature communications **12**, 1 (2021).

[6] A. Ciarrocchi, D. Unuchek, A. Avsar, K. Watanabe, T. Taniguchi, and A. Kis, Polarization switching and electrical control of interlayer excitons in two-dimensional van der waals heterostructures, Nature photonics **13**, 131 (2019).

[7] A. Delhomme, D. Vaclavkova, A. Slobodeniuk, M. Orlita, M. Potemski, D. Basko, K. Watanabe, T. Taniguchi, D. Mauro, C. Barreteau, *et al.*, Flipping exciton angular momentum with chiral phonons in mose2/wse2 heterobilayers, 2D Materials **7**, 041002 (2020).

[8] T. Wang, S. Miao, Z. Li, Y. Meng, Z. Lu, Z. Lian, M. Blei, T. Taniguchi, K. Watanabe, S. Tongay, *et al.*, Giant valley-zeeman splitting from spin-singlet and spin-triplet interlayer excitons in wse2/mose2 heterostructure, Nano letters **20**, 694 (2019).

[9] E. Calman, L. Fowler-Gerace, D. Choksy, L. Butov, D. Nikonov, I. Young, S. Hu, A. Mishchenko, and A. Geim, Indirect excitons and trions in mose2/wse2 van der waals heterostructures, Nano Letters **20**, 1869 (2020).

[10] E. Barré, O. Karni, E. Liu, A. L. O'Beirne, X. Chen, H. B. Ribeiro, L. Yu, B. Kim, K. Watanabe, T. Taniguchi, *et al.*, Optical absorption of interlayer excitons in transition-metal dichalcogenide heterostructures, Science **376**, 406 (2022).

[11] L.-Y. Gan, Q. Zhang, Y.-J. Zhao, Y. Cheng, and U. Schwingenschlögl, Order-disorder phase transitions in the two-dimensional semiconducting transition metal dichalcogenide alloys mo1- xwxx2 (x= s, se and te), Scientific reports **4**, 1 (2014).

[12] E. M. Alexeev, D. A. Ruiz-Tijerina, M. Danovich, M. J. Hamer, D. J. Terry, P. K. Nayak, S. Ahn, S. Pak, J. Lee, J. I. Sohn, *et al.*, Resonantly hybridized excitons in moiré superlattices in van der waals heterostructures, Nature **567**, 81 (2019).

[13] D. A. Ruiz-Tijerina and V. I. Fal'ko, Interlayer hybridization and moiré superlattice minibands for electrons and excitons in heterobilayers of transition-metal dichalcogenides, Phys. Rev. B **99**, 125424 (2019).

[14] S. J. Magorrian, V. V. Enaldiev, V. Zólyomi, F. Ferreira, V. I. Fal'ko, and D. A. Ruiz-Tijerina, Multifaceted moiré superlattice physics in twisted $wse_2$ bilayers, Phys. Rev. B **104**, 125440 (2021).

[15] A. Weston, Y. Zou, V. Enaldiev, A. Summerfield, N. Clark, V. Zólyomi, A. Graham, C. Yelgel, S. Magorrian, M. Zhou, *et al.*, Atomic reconstruction in twisted bilayers of transition metal dichalcogenides, Nature Nanotechnology **15**, 592 (2020).

[16] M. R. Rosenberger, H.-J. Chuang, M. Phillips, V. P. Oleshko, K. M. McCreary, S. V. Sivaram, C. S. Hellberg, and B. T. Jonker, Twist angle-dependent atomic reconstruction and moiré patterns in transition metal dichalcogenide heterostructures, ACS nano **14**, 4550 (2020).
